# Supplementary material for: High-energy magnetic excitations in Bi$_2$Sr$_2$CaCu$_2$O$_{8+\delta}$: Towards a unified description of the electronic and magnetic degrees of freedom in the cuprates
Source: arXiv:1212.3714 source file (2013-02-21)
Supplement: Supplementary file 1 [file supplementary.pdf]

# Supplementary Material for: High-energy magnetic excitations in $\text{Bi}_2\text{Sr}_2\text{CaCu}_2\text{O}_{8+\delta}$ : Towards a unified description of its electronic and magnetic degrees of freedom

(Dated: February 11, 2013)

Here we provide an additional diagram depicting the scattering geometry, a more detailed description of the fitting of the RIXS spectra and further details of our parameterization of the  $\text{Bi}_2\text{Sr}_2\text{CaCu}_2\text{O}_{8+\delta}$  electronic structure according to the Yang-Rice-Zhang ansatz (YRZ) [1]. Then we go on to describe how this provides a basis for calculating the magnetic response.

## EXPERIMENTAL GEOMETRY

Figure 1 shows further details of the scattering geometry used in the experiment. In addition to the parameters defined in the main text, here we define the total momentum transfer  $\mathbf{Q}$ , which is resolved into  $Q_{\parallel}$ , parallel to  $a^*$ , and  $Q_{\perp}$ , parallel to  $c^*$ .  $\delta$  is the angle between  $\mathbf{Q}$  and  $Q_{\perp}$ . In this diagram  $\pi$ -incident x-rays have polarization in the plane of the diagram perpendicular to  $\mathbf{k}_i$  and  $\sigma$ -incident x-rays have polarization perpendicular to the plane of the diagram. The ADDRESS beamline used for these measurements employs an APPLE-II type helical undulator which produces highly ( $\sim 99\%$ ) polarized x-rays.

## FITTING THE RIXS SPECTRA

As described in several studies of the cuprates (see for example Refs. [2–6]) several different types of scattering processes are present in Cu  $L_3$  edge RIXS spectra. These include elastic processes from specular and diffuse scattering, phonons below  $\sim 90$  meV, single spin-flip scattering, multi spin-flip scattering, charge scattering and orbital scattering. All the peaks used in the fitting here and in previous work [4] were convolved with a Gaussian function, which is an excellent approximation to the resolution function of the SAXES instrument used in this study. By definition, the elastic scattering is a  $\delta$ -function at 0 eV energy transfer, which leads to a Gaussian when convolved with the resolution function. The electronic and orbital scattering causes a tail of scattering in the low energy region, which can be modeled by a smooth function, and in this case we used a third order polynomial. In YBCO (Ref. 4) the RIXS spectrum could be fit with a resolution-limited Gaussian to account for the elastic line, an anti-symmetrized Lorentzian to account for the phonon, single spin-flip paramagnon and multi spin-flip scattering and a smooth background. In Bi-2212 we find that the low energy inelastic scattering cannot be adequately accounted for with an anti-symmetrized Lorentzian as the high energy tail of the

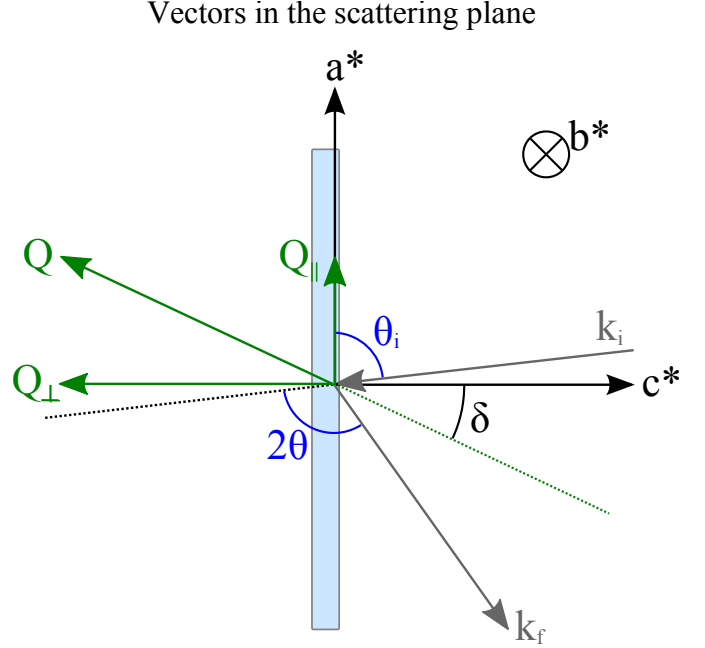

FIG. 1. (Color online) The scattering geometry in the  $ac$ -plane showing the definitions of the different angles and vectors used in the experiment.  $\mathbf{k}_i$  and  $\mathbf{k}_f$  are the initial and final scattering vectors of the x-rays.  $2\theta = 130^\circ$  is the angle between  $\mathbf{k}_i$  and  $\mathbf{k}_f$ .  $\theta_i$  is the angle between the sample surface and  $\mathbf{k}_i$ .  $a^*$  and  $c^*$  are the reciprocal lattice vectors.  $\mathbf{Q}$  is the total momentum transfer, which is resolved into  $Q_{\parallel}$ , parallel to  $a^*$ , and  $Q_{\perp}$ , parallel to  $c^*$ .

paramagnon extends out too far in energy. Similarly, a measurement of  $\text{La}_{1.92}\text{Sr}_{0.08}\text{CuO}_4$  also could not account for the low energy inelastic scattering in terms of a single anti-symmetrized Lorentzian [3]. Given that the phonon, single spin-flip and multi spin-flip scattering in Bi-2212 could not be unambiguously separated, we used an anti-symmetrized Lorentzian plus two Gaussians to provide a smooth line, which accounts for the MIR region of the RIXS spectrum. In essence, however, this is a phenomenological method to provide a smooth line within the confidence limits set by twice the errorbars. The paramagnon energy is taken to be the peak of this smooth line. The error is estimated by adding the uncertainty in the fit procedure to the uncertainty in determining the zero energy transfer energy via scattering from carbon tape.

# YRZ PARAMETERIZATION OF THE ELECTRONIC STRUCTURE OF Bi-2212

In the YRZ model the coherent single particle excitations are described by a Green's function for spinons

$$G(\omega, \mathbf{k}) = \frac{1}{\omega - \xi(\mathbf{k}) - \Sigma_R(\omega, \mathbf{k})}, \quad (1)$$

where  $\xi(\mathbf{k})$  is a hopping dispersion (including terms up to next-next-nearest neighbor) renormalized by doping

$$\xi(\mathbf{k}) = \xi_0(\mathbf{k}) + \xi'(\mathbf{k}), \quad (2a)$$

$$\xi_0(\mathbf{k}) = -2t(x)(\cos k_x + \cos k_y), \quad (2b)$$

$$\xi'(\mathbf{k}) = -4t'(x) \cos k_x \cos k_y - 2t''(x)(\cos 2k_x + \cos 2k_y) - \mu_p, \quad (2c)$$

and

$$\Sigma_R(\omega, \mathbf{k}) = |\Delta_R(\mathbf{k})|^2 / [\omega + \xi_0(\mathbf{k})], \quad (3)$$

is a self energy term that depends on the pseudogap

$$\Delta_R(\mathbf{k}) = \Delta_0(x)(\cos k_x - \cos k_y). \quad (4)$$

The doping dependence is included via Gutzwiller factors [7],

$$g_t = \frac{2x}{1+x}, \quad (5a)$$

$$g_s = \frac{4}{(1+x)^2}, \quad (5b)$$

which renormalize the bare hopping and exchange parameters  $t_0$ ,  $t'_0$ ,  $t''_0$  and  $J$ :

$$t(x) = g_t t_0 + \frac{3}{8} g_s J \chi, \quad (5c)$$

$$t'(x) = g_t t'_0, \quad (5d)$$

$$t''(x) = g_t t''_0, \quad (5e)$$

with  $\chi = 0.338$  [8]. The bare parameters arise from an underlying  $t - J$  Hamiltonian description

$$H_{t-J} = P_s \left( - \sum_{ijs} t_{0,ij} c_{is}^\dagger c_{js} + J \sum_{\langle ij \rangle} \mathbf{S}_i \cdot \mathbf{S}_j \right) P_s, \quad (6)$$

where  $P_s$  is a projection operator onto the singly occupied subspace. Note that the exchange  $J$  enters the dispersion as a hopping-like term due to a mean field factorization of the spin interaction [1].

The precise form of the pseudogap in the cuprates is still an issue of debate, especially the question of whether the pseudogap closes at optimal doping or in the overdoped regime where superconductivity disappears [9, 10]. The original formulation of YRZ assumed the former [1] but ARPES measurements tend to side with the latter scenario [10] and indeed this is the finding of ARPES measurements on Bi-2212 samples made in the same way

TABLE I. The bare parameters.

| $t_0$    | $t'_0$    | $t''_0$  | $J$     | $\chi$ | $\Delta_0$ |
|----------|-----------|----------|---------|--------|------------|
| $3J/2.5$ | $-0.3t_0$ | $0.2t_0$ | 0.12 eV | 0.338  | $0.3t_0$   |

as the sample we study here [11]. Given that our aim is to reconcile ARPES measurements of the electronic structure of Bi-2212 with our RIXS measurements of the magnetic excitations, we follow the convention of Ref. [11]. Namely we choose a simple linearly decreasing phenomenological form for the pseudogap

$$\Delta_0(x) = \Delta_0(1 - x/x_{\text{crit}}), \quad (7)$$

which disappears at  $x_{\text{crit}} = 0.20$ , the overdoped edge of the superconducting dome [12]. The overall magnitude,  $\Delta_0$ , is chosen by fitting to the measured electronic structure [11] as explained later. We note that our results are not highly sensitive to the precise value of  $x_{\text{crit}}$ .

ARPES, when corrected for matrix element effects and divided by the Fermi occupation factor, measures the spectral function  $A(\mathbf{k}, \omega)$ , which is directly related to the Green's function as  $A(\mathbf{k}, \omega) = -(1/\pi) \text{Im} G(\mathbf{k}, \omega)$ . This relationship was used in [11] to determine the parameters for the YRZ model applied to  $\text{Bi}_2\text{Sr}_2\text{CaCu}_2\text{O}_{8+\delta}$ . Table I shows this bare parameter set [12]. As emphasized in the text, we use the doping values obtained in the fitting of the ARPES data: For the underdoped sample  $x = 0.03$  and at optimal doping  $x = 0.16$ . The chemical potential,  $\mu_p$  is set according to Luttinger's sum rule [1] self consistently and found to be -0.036 and -0.054 for  $x = 0.03$  and 0.16 respectively. We plot the resulting YRZ forms for the electronic structure of Bi-2212 in Fig. 2.

Unfortunately, the YRZ ansatz in its original form is a single particle Green's function and does not constitute a starting point for calculating the magnetic response. However, a slave boson treatment of the  $t - J$  model, in which fermionic 'spinons' are bound to bosonic 'holons' reproduces the YRZ propagator [13]. This provides a connection to standard many body theoretical techniques [14, 15]: one can calculate  $S(\mathbf{Q}, \omega)$  via a resummation of particle-hole bubble diagrams [14].

The YRZ ansatz factors into two effective bands and can be extended to include superconductivity by treating the system as a two band superconductor [16]. We write the superconducting gap in the  $i$  band as  $\Delta_{s,i}(\mathbf{k}) = \Delta_{s,i}(x)[\cos(k_x) - \cos(k_y)]$ . Because the upper, (+), YRZ band is far above the Fermi energy we set  $\Delta_{s,+} = 0$  and take  $\Delta_{s,-} = 0.07t_0(1 - 91(x - x_{\text{crit}})^2)$  in the superconducting state [11, 12]. In the heavily underdoped, non-superconducting case  $\Delta_{s,+} = \Delta_{s,-} = 0$ . The propagator is then written as a Nambu-Gor'kov (matrix) Green's function (with momentum labels suppressed and Pauli

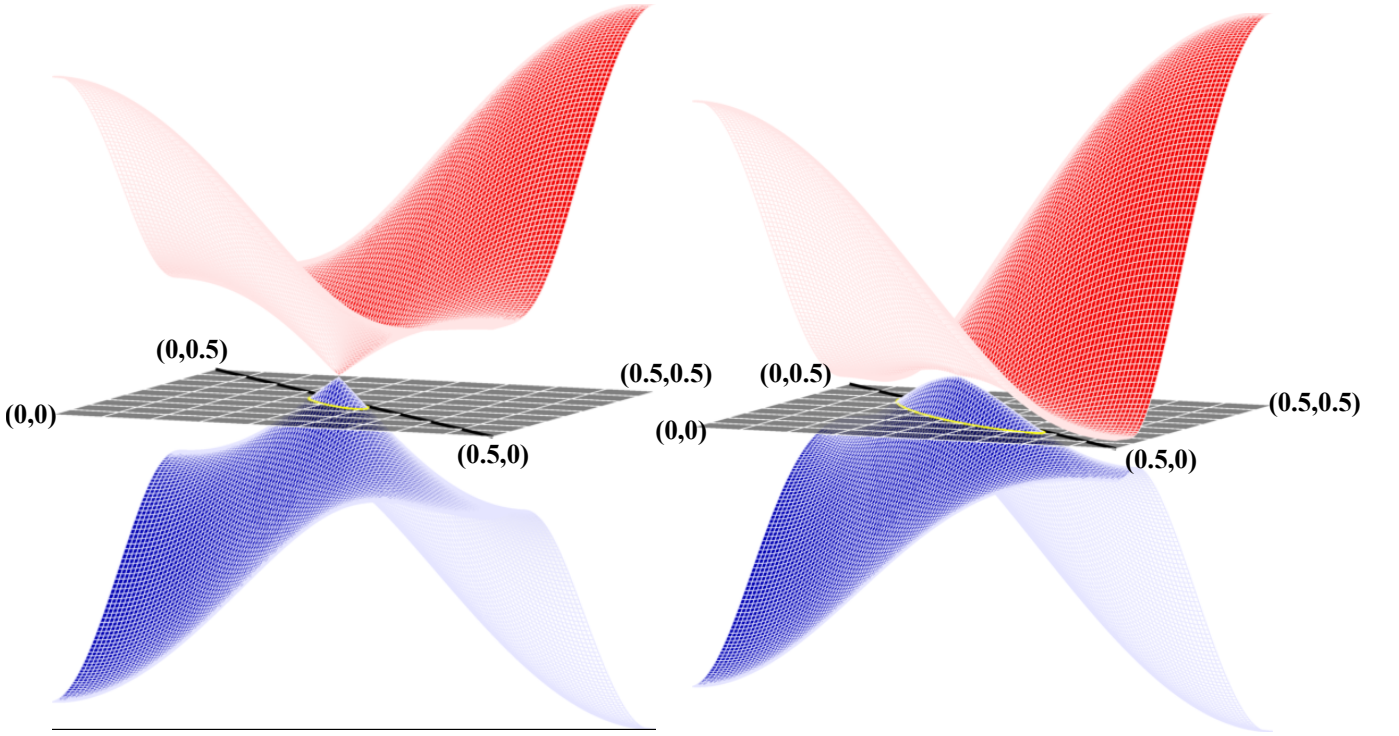

FIG. 2. (Color online) The YRZ form for the electronic structure of Bi-2212, which produces two effective bands with the Fermi energy lying in the lower band. The resulting Fermi surface consists of hole pockets, with an area proportional to doping. The intensity of color is proportional to the coherent quasi-particle weight. The lower, blue band has strong quasi-particle weight on the side near  $(0,0)$  and weak quasi-particle weight on the far side towards  $(0.5,0.5)$ . The gray surface represents the Fermi energy, which forms the Fermi surface outlined in yellow. The gap between the upper and lower bands closes along the Brillouin zone diagonal  $(0,0) \rightarrow (0.5,0.5)$  at the top of the pocket. A key feature of the YRZ model is that the quasiparticle weight vanishes at the back of the pockets. The left hand plot shows the bands for the underdoped,  $x = 0.03$  case and the right hand plot shows the optimally,  $x = 0.16$ , doped case.

matrices  $\tau$ )

$$\mathbf{G}^s(\omega, \mathbf{k}) = \sum_{i=\pm} z_i \frac{\omega \tau_0 + \omega_i(\mathbf{k}) \tau_z - \Delta_{s,i}(\mathbf{k}) \tau_x}{\omega^2 - \omega_i^2(\mathbf{k}) - \Delta_{s,i}^2(\mathbf{k})}, \quad (8)$$

with

$$\begin{aligned} \omega_{\pm} &= \frac{\xi'(\mathbf{k})}{2} \pm \sqrt{\bar{\xi}(\mathbf{k})^2 + \Delta_R^2(\mathbf{k})}, \\ z_{\pm}(\mathbf{k}) &= \frac{1}{2} \pm \frac{\bar{\xi}(\mathbf{k})}{2\sqrt{\bar{\xi}(\mathbf{k})^2 + \Delta_R^2(\mathbf{k})}}, \end{aligned} \quad (9)$$

and we have defined  $\bar{\xi}(\mathbf{k}) = [\xi(\mathbf{k}) + \xi_0(\mathbf{k})]/2$ .

The lowest order contribution to the magnetic response at  $T = 0$  is

$$\begin{aligned} \Pi^s(\omega, \mathbf{Q}) &= \int \frac{d\mathbf{k}}{(2\pi)^2} \sum_{ij=\pm} \frac{z_i(\mathbf{k}) z_j(\mathbf{k} + \mathbf{Q})}{8} \left( 1 \right. \\ &\quad \left. - \frac{\omega_i(\mathbf{k}) \omega_j(\mathbf{k} + \mathbf{Q}) + \Delta_{s,i}(\mathbf{k}) \Delta_{s,j}(\mathbf{k} + \mathbf{Q})}{E_{s,i}(\mathbf{k}) E_{s,j}(\mathbf{k} + \mathbf{Q})} \right) \\ &\quad \times \left[ \frac{1}{\omega - E_{s,j}(\mathbf{k} + \mathbf{Q}) - E_{s,i}(\mathbf{k})} \right. \\ &\quad \left. - \frac{1}{\omega + E_{s,j}(\mathbf{k} + \mathbf{Q}) + E_{s,i}(\mathbf{k})} \right], \end{aligned} \quad (10)$$

where

$$E_{s,i}(\mathbf{k}) = \sqrt{\omega_i^2(\mathbf{k}) + \Delta_{s,i}^2(\mathbf{k})}. \quad (11)$$

On setting  $\Delta_s = 0$  one recovers the  $T = 0$  normal state particle-hole bubble diagram, composed of YRZ propagators. We evaluate  $\Pi_s(\omega, \mathbf{Q})$  numerically by summing over a grid of  $1000 \times 1000$  points in  $\mathbf{k}$  space.

The dynamical structure factor is given by the RPA resummation

$$S(\mathbf{Q}, \omega) = -\frac{1}{\pi} \lim_{\eta \rightarrow 0} \text{Im} \frac{\Pi^s(\omega + i\eta, \mathbf{Q})}{1 - \tilde{J}(\mathbf{Q}) \Pi^s(\omega + i\eta, \mathbf{Q})}, \quad (12)$$

with an antiferromagnetic exchange  $\tilde{J}(\mathbf{Q}) = 2\tilde{J}(\cos Q_x + \cos Q_y)$ . Here we write  $\tilde{J}$  to indicate that the bare exchange  $J$  that appears in Eq. 6 should be renormalized by higher order terms (such as interactions between holes and spin excitations that disrupt antiferromagnetic correlations) [14]. The neglect of these higher order terms is a limitation of our approach. In fact in Ref. [14] the necessary renormalization factor was found to be quite large,  $\sim 1/3$ , in order to produce the transition to antiferromagnetic order at a low doping. Treating  $\tilde{J}$  as a fitting

parameter for the  $\sim 40$  meV resonance measured at optimal doping ( $x = 0.16$ ) we find  $\tilde{J} = 135$  meV, compared to  $J = 120$  meV. Further discussion of these issues can be found in Ref. [13]. For the energies and wave vectors relevant to the RIXS data presented in this work the resummation is negligible. It does however have some effect at low energies near  $(0, 0)$ , causing a small broadening in energy. Inserting the numerically evaluated bubble, Eq. 10, into Eq. 12 we arrive at the theoretical results for the magnetic response shown in Fig 3. of the letter.

- 
- [1] K.-Y. Yang, T. M. Rice, and F.-C. Zhang, Phys. Rev. B **73**, 174501 (2006).
  - [2] L. Braicovich, L. J. P. Ament, V. Bisogni, F. Forte, C. Aruta, G. Balestrino, N. B. Brookes, G. M. D. Luca, P. G. Medaglia, F. M. Granozio, M. Radovic, M. Salluzzo, J. V. D. Brink, and G. Ghiringhelli, Phys. Rev. Lett. **167401**, 22 (2009).
  - [3] L. Braicovich, J. van den Brink, V. Bisogni, M. M. Sala, L. J. P. Ament, N. B. Brookes, G. M. De Luca, M. Salluzzo, T. Schmitt, V. N. Strocov, and G. Ghiringhelli, Phys. Rev. Lett. **104**, 077002 (2010).
  - [4] M. Le Tacon, G. Ghiringhelli, J. Chaloupka, M. M. Sala, V. Hinkov, M. W. Haverkort, M. Minola, M. Bakr, K. J. Zhou, S. Blanco-Canosa, C. Monney, Y. T. Song, G. L. Sun, C. T. Lin, G. M. De Luca, M. Salluzzo, G. Khal-iullin, T. Schmitt, L. Braicovich, and B. Keimer, Nat Phys **7**, 725 (2011).
  - [5] L. J. P. Ament, M. van Veenendaal, T. P. Devereaux, J. P. Hill, and J. van den Brink, Rev. Mod. Phys. (2011).
  - [6] M. P. M. Dean, R. S. Springell, C. Monney, K. J. Zhou, J. Pereiro, I. Božović, B. Dalla Piazza, H. M. Rønnow, E. Morenzoni, J. van den Brink, T. Schmitt, and J. P. Hill, Nature Materials **11**, 850 (2012).
  - [7] M. C. Gutzwiller, Phys. Rev. Lett. **10**, 159 (1963).
  - [8] F. C. Zhang, C. Gros, T. M. Rice, and H. Shiba, Superconductor Science and Technology **1**, 36 (1988).
  - [9] M. R. Norman, D. Pines, and C. Kallin, Advances in Physics **54**, 715 (2005).
  - [10] T. Yoshida, M. Hashimoto, I. M. Vishik, Z.-X. Shen, and A. Fujimori, Journal of the Physical Society of Japan **81**, 011006 (2012).
  - [11] H.-B. Yang, J. D. Rameau, Z.-H. Pan, G. D. Gu, P. D. Johnson, H. Claus, D. G. Hinks, and T. E. Kidd, Phys. Rev. Lett. **107**, 047003 (2011).
  - [12] J. Rameau, (2012), private communication.
  - [13] A. J. A. James, R. M. Konik, and T. M. Rice, Phys. Rev. B **86**, 100508 (2012).
  - [14] J. Brinckmann and P. A. Lee, Phys. Rev. B **65**, 014502 (2001).
  - [15] A. Altland and B. D. Simons, *Condensed Matter Field Theory* (Cambridge University Press, 2010).
  - [16] K.-Y. Yang, H.-B. Yang, P. D. Johnson, T. M. Rice, and F.-C. Zhang, EPL (Europhysics Letters) **86**, 37002 (2009).
